# Supplementary material for: Improved methods for empirical Bayes multivariate multiple testing and effect size estimation
Source: arXiv:2406.08784 ancillary file (2024-06-13)
Supplement: Supplementary file 1 [file supplementary_materials.pdf]

*Submitted to the Annals of Applied Statistics*

# SUPPLEMENTARY MATERIALS FOR "IMPROVED METHODS FOR EMPIRICAL BAYES MULTIVARIATE MULTIPLE TESTING AND EFFECT SIZE ESTIMATION"

BY YUNQI YANG[1], PETER CARBONETTO[2]
DAVID GERARD[3] AND MATTHEW STEPHENS[2,4,a]

[1]*Committee on Genetics, Genomics and System Biology, University of Chicago*

[2]*Department of Human Genetics, University of Chicago*

[3]*Department of Mathematics and Statistics, American University*

[4]*Department of Statistics, University of Chicago,* [a]*mstephens@uchicago.edu*

## 1. Derivations, proofs, and additional definitions.

1.1. *Posterior distribution for unknown means.* Urbut et al. (2019) gives the posterior distributions only for the case when the prior covariances $\boldsymbol{U}_k$ are invertible, so here we give the slightly more general expressions that allow for one or more of the $\boldsymbol{U}_k$ to be singular.

For $\boldsymbol{x} \mid \boldsymbol{\theta} \sim N_R(\boldsymbol{\theta}, \boldsymbol{V})$ and $\boldsymbol{\theta} \sim N_R(\boldsymbol{0}, \boldsymbol{U})$, we have

$$\boldsymbol{\theta} \mid \boldsymbol{x} \sim N_R(\boldsymbol{\mu}^*, \boldsymbol{U}^*) \tag{30}$$

in which

$$\boldsymbol{U}^* := \boldsymbol{U}^*(\boldsymbol{U}, \boldsymbol{V}) = \boldsymbol{U}(\boldsymbol{I}_R + \boldsymbol{V}^{-1}\boldsymbol{U})^{-1} \tag{31}$$

$$\boldsymbol{\mu}^* := \boldsymbol{\mu}^*(\boldsymbol{U}, \boldsymbol{V}, \boldsymbol{x}) = \boldsymbol{U}^*\boldsymbol{V}^{-1}\boldsymbol{x}. \tag{32}$$

For the mixture prior, the posterior distribution is

$$p(\boldsymbol{\theta}_j \mid \boldsymbol{x}_j, \boldsymbol{\pi}, \mathcal{U}) = \sum_{k=1}^{K} \pi_{jk}^* N_R(\boldsymbol{\theta}_j; \boldsymbol{\mu}_{jk}^*, \boldsymbol{U}_{jk}^*) \tag{33}$$

where $\boldsymbol{U}_{jk}^* := \boldsymbol{U}^*(\boldsymbol{U}_k, \boldsymbol{V}_j)$ and $\boldsymbol{\mu}_{jk}^* := \boldsymbol{\mu}^*(\boldsymbol{U}_k, \boldsymbol{V}_j, \boldsymbol{x}_j)$, and

$$\pi_{jk}^* := \frac{\pi_k N_R(\boldsymbol{x}_j; 0, \boldsymbol{U}_k + \boldsymbol{V}_j)}{\sum_{k'=1}^{K} \pi_{k'} N_R(\boldsymbol{x}_j; 0, \boldsymbol{U}_{k'} + \boldsymbol{V}_j)}. \tag{34}$$

These expressions are the same as the expressions in Urbut et al. (2019) when all the $\boldsymbol{U}_k$ are invertible.

1.2. *EM for weighted log-likelihoods.* In this section we derive an "EM-like" algorithm for maximizing a weighted log-likelihood of the form:

$$\begin{aligned}\phi(\Theta; \boldsymbol{w}) &:= \sum_{j=1}^{n} w_j \log p_j(\boldsymbol{x}_j \mid \Theta) \\ &= \sum_{j=1}^{n} w_j l_j(\Theta), \end{aligned} \tag{35}$$

where the $w_j$ are known (fixed) weights, the $\boldsymbol{x}_j$ denote the independently observed data, and $\Theta$ denotes the unknowns to be estimated. Note that here we do not make specific modeling assumptions; in particular, the results are not specific to the EBMNM model.

We assume, as in usual applications of EM, that the likelihoods can be written using an "augmented data" form; that is, $p_j(\boldsymbol{x}_j \mid \Theta) = \int p_j(\boldsymbol{x}_j, \boldsymbol{z}_j \mid \Theta)\, d\boldsymbol{z}_j$.

The following proposition gives an "EM-like" update that is guaranteed to increase (or not decrease) the weighted log-likelihood, $\phi$.

PROPOSITION 1. Given the current value of $\Theta$, denoted $\Theta^{(0)}$, define a new value, $\Theta^{(1)}$, by applying the following steps:

1. E-step: For each $j = 1, \dots, n$, compute the conditional distribution of $\boldsymbol{z}_j$, $p_j(\boldsymbol{z}_j \mid \boldsymbol{x}_j, \Theta^{(0)})$.

2. M-step: Set $\Theta^{(1)} = \text{argmax}_\Theta \sum_{j=1}^n w_j \mathrm{E}_{p_j(\boldsymbol{z}_j \mid \boldsymbol{x}_j, \Theta^{(0)})}\big[\log p(\boldsymbol{x}_j, \boldsymbol{z}_j \mid \Theta)\big]$.

Then $\phi(\Theta^{(1)}; \boldsymbol{w}) \geq \phi(\Theta^{(0)}; \boldsymbol{w})$.

Note that when the weights $w_j$ are all 1, these steps are the standard E-step and M-step in EM.

PROOF. Following Neal and Hinton (1998), we define

$$F(q_1, \dots, q_n; \Theta) := \sum_{j=1}^n w_j \big\{ \mathrm{E}_{q_j}[\log p_j(\boldsymbol{x}_j, \boldsymbol{z}_j \mid \Theta)] + H(q_j) \big\}, \tag{36}$$

where $q_j$ is any distribution of $\boldsymbol{z}_j$ and $H(q_j) = -\mathrm{E}_{q_j}[\log q_j(\boldsymbol{z}_j)]$ is the entropy of distribution $q_j$. Using Lemma 1, 2 of Neal and Hinton (1998), we have

$$\hat{q}_j(\Theta) := \text{argmax}_{q_j} F(q_1, \dots, q_n; \Theta) = p_j(\boldsymbol{z}_j \mid \boldsymbol{x}_j, \Theta), \quad j = 1, \dots, n. \tag{37}$$

$$F(\hat{q}(\Theta); \Theta) = \sum_{j=1}^n w_j l_j(\Theta) = \phi(\Theta; \boldsymbol{w}), \tag{38}$$

where we have introduced the notation $\hat{q}(\Theta)$ as shorthand for $\hat{q}_1(\Theta), \dots, \hat{q}_n(\Theta)$.

The function being maximized in the M-step differs from $F(\hat{q}(\Theta^{(0)}); \Theta)$ only by terms that do not depend on $\Theta$, so the M-step can be written as

$$\Theta^{(1)} = \text{argmax}_\Theta F(\hat{q}(\Theta^{(0)}); \Theta). \tag{39}$$

Therefore,

$$\phi(\Theta^{(1)}; \boldsymbol{w}) = F(\hat{q}(\Theta^{(1)}), \Theta^{(1)}) \geq F(\hat{q}(\Theta^{(0)}), \Theta^{(1)}) \geq F(\hat{q}(\Theta^{(0)}), \Theta^{(0)}) = \phi(\Theta^{(0)}; \boldsymbol{w}),$$

where the equalities are due to (38); the first inequality is due to the optimality of $\hat{q}(\Theta^{(1)})$ from its definition, and the second inequality is due to the optimality of $\Theta^{(1)}$ in (39). This completes the proof.

□

1.3. *Derivation of the EM algorithm for fitting the EBMNM model.* Here we derive the general EM algorithm for EBMNM (Algorithm 1).

First, we introduce a latent variable $\boldsymbol{z}_j$ for each $j = 1, \dots, n$. Each $\boldsymbol{z}_j$ is a binary vector of length $K$ indicating the component $k$ from which $\boldsymbol{x}_j$ arose. Following Neal and Hinton (1998), we introduce the function $F(q, \mathcal{U}, \boldsymbol{\pi}, \boldsymbol{s})$,

(40)

$$\begin{aligned} F(q, \mathcal{U}, \boldsymbol{\pi}, \boldsymbol{s}) &= E_q[\log p(\boldsymbol{x}, \boldsymbol{z}; \mathcal{U}, \boldsymbol{\pi}) - \textstyle\sum_{k=1}^K \rho(\boldsymbol{U}_k / s_k)] - E_q[\log q(\boldsymbol{z})] \\ &= \sum_{j=1}^n \sum_{k=1}^K E_q\big[\log(\pi_k) + \log N_R(\boldsymbol{x}_j; 0, \boldsymbol{U}_k + \boldsymbol{V}_j)\big] - \sum_{k=1}^K \rho(\boldsymbol{U}_k / s_k) - E_q[\log q(\boldsymbol{z})], \end{aligned}$$

where $q$ is any distribution over $\boldsymbol{z}$. Note that the only difference between (40) and the function $F$ in Neal and Hinton (1998) is a constant term with respect to $q$, the penalty $\sum_{k=1}^{K} \rho(\boldsymbol{U}_k/s_k)$. Therefore, we can use Lemma 1 and Lemma 2 in Neal and Hinton (1998), which shows that the log-likelihood is related to $F$ by

$$F(\hat{q}, \mathcal{U}, \boldsymbol{\pi}, \boldsymbol{s}) = l(\mathcal{U}, \boldsymbol{\pi}, \boldsymbol{s}), \tag{41}$$

where $\hat{q} := \operatorname{argmax}_q F(q, \mathcal{U}, \boldsymbol{\pi}, \boldsymbol{s})$, and is the conditional distribution of $\boldsymbol{z}$,

$$\hat{q}(\boldsymbol{z}) := \operatorname{argmax}_q F(q, \mathcal{U}, \boldsymbol{\pi}) = p(\boldsymbol{z} \mid \boldsymbol{x}, \mathcal{U}, \boldsymbol{\pi}). \tag{42}$$

In our case, $F$ is related to the penalized log-likelihood,

$$F(\hat{q}, \boldsymbol{s}, \mathcal{U}, \boldsymbol{\pi}) = l(\mathcal{U}, \boldsymbol{\pi}) - \sum_{k=1}^{K} \rho(\boldsymbol{U}_k/s_k). \tag{43}$$

Therefore, the maximum-likelihood estimates of $\boldsymbol{s}, \boldsymbol{\pi}$ and the penalized maximum-likelihood estimates of $\boldsymbol{U}$ can be obtained by maximizing $F$ jointly over $q, \boldsymbol{s}, \boldsymbol{U}, \boldsymbol{\pi}$:

$$\begin{aligned}(\hat{\mathcal{U}}, \hat{\boldsymbol{\pi}}, \hat{\boldsymbol{s}}) &:= \operatorname{argmax}_{\boldsymbol{s}, \mathcal{U}, \boldsymbol{\pi}} l(\mathcal{U}, \boldsymbol{\pi}) - \textstyle\sum_{k=1}^{K} \rho(\boldsymbol{U}_k/s_k) \\ &= \operatorname{argmax}_{\boldsymbol{s}, \mathcal{U}, \boldsymbol{\pi}} \max_q F(q, \mathcal{U}, \boldsymbol{\pi}, \boldsymbol{s}).\end{aligned}$$

The standard EM algorithm can be thought of as iterating between optimizing over $q$ (the E-step) and optimizing over $\mathcal{U}, \boldsymbol{\pi}, \boldsymbol{s}$ (the M-step). The E-step computes $\hat{q}$. The expected value of $z_{jk}$ under $\hat{q}$ is

$$w_{jk} := E_{\hat{q}}[z_{jk}] = \frac{\pi_k N_R(\boldsymbol{x}_j; 0, \boldsymbol{U}_k + \boldsymbol{V}_j)}{\sum_{k'=1}^{K} \pi_{k'} N_R(\boldsymbol{x}_j; 0, \boldsymbol{U}_{k'} + \boldsymbol{V}_j)}. \tag{44}$$

The part of the M-Step optimizing $F$ over $\boldsymbol{\pi}$ is straightforward and given by

$$\hat{\pi}_k = \frac{1}{n} \sum_{j=1}^{n} w_{jk}, \quad k = 1, \ldots, K. \tag{45}$$

Optimizing $F$ over $\boldsymbol{U}_k$ and $s_k$ is described below.

1.4. *Data transformation for homoskedastic case of EBMNM.* When $\boldsymbol{V}_j = \boldsymbol{V}$, we can simplify the fitting procedure of EBMNM model by performing a data transformation and then applying algorithms to the case of $\boldsymbol{V} = \boldsymbol{I}_R$ on transformed data. Here we describe this approach in more details.

Let $\boldsymbol{R}$ be any matrix such that $\boldsymbol{V} = \boldsymbol{R}\boldsymbol{R}^T$ (e.g., $\boldsymbol{R}$ could be the Cholesky decomposition of $\boldsymbol{V}$). Since $\boldsymbol{V}$ is invertible, $\boldsymbol{R}$ is also invertible, so consider the transformed data $\tilde{\boldsymbol{x}}_j := \boldsymbol{R}^{-1}\boldsymbol{x}_j$. The marginal model (3) for the transformed data becomes

$$p(\tilde{\boldsymbol{x}}_j \mid \boldsymbol{\pi}, \mathcal{U}, \boldsymbol{V}_j) = \sum_{k=1}^{K} \pi_k N_R(\tilde{\boldsymbol{x}}_j; \boldsymbol{0}, \tilde{\boldsymbol{U}}_k + \boldsymbol{I}_R), \tag{46}$$

where $\tilde{\boldsymbol{U}}_k := \boldsymbol{R}^{-1}\boldsymbol{U}_k\boldsymbol{R}^{-T}$. Thus, we can estimate $\boldsymbol{U}_k$ by first estimating $\tilde{\boldsymbol{U}}_k$—by fitting the EBMNM model to transformed data $\tilde{\boldsymbol{x}}_j$ with $\boldsymbol{V} = \boldsymbol{I}_R$, yielding estimates $\hat{\tilde{\boldsymbol{U}}}_k$ say—and then reversing the transformation to obtain estimates $\hat{\boldsymbol{U}}_k$ for $\boldsymbol{U}_k$,

$$\hat{\boldsymbol{U}}_k = \boldsymbol{R}\hat{\tilde{\boldsymbol{U}}}_k\boldsymbol{R}^T, \quad k = 1, \ldots, K. \tag{47}$$

When taking this approach, any constraint on $\boldsymbol{U}_k$ ($\boldsymbol{U}_k \in P_R^{+,k}$) must be translated to an equivalent corresponding constraint on $\tilde{\boldsymbol{U}}_k$ ($\tilde{\boldsymbol{U}}_k \in \tilde{P}_R^{+,k}$ say) when fitting the EBMNM model. For example, a rank-1 constraint on $\boldsymbol{U}_k$ translates to a rank-1 constraint on $\tilde{\boldsymbol{U}}$.

Note that with this transformation, when a penalty function is included in the EBMNM problem, the penalty is imposed on $\tilde{\boldsymbol{U}}_k$ rather than on $\boldsymbol{U}_k$. Specifically, it can be shown that this transformation approach, instead of solving (9), solves

$$(\hat{\boldsymbol{\pi}}, \hat{\mathcal{U}}, \hat{\boldsymbol{s}}) := \operatorname*{argmax}_{\boldsymbol{\pi} \in \boldsymbol{S}_K, \boldsymbol{U}_k \in P_R^{+,k}} l(\boldsymbol{\pi}, \mathcal{U}) - \min_{\boldsymbol{s}} \sum_{k=1}^{K} \rho\left(\boldsymbol{R}^{-1}\boldsymbol{U}_k\boldsymbol{R}^{-T}/s_k\right). \tag{48}$$

When no penalty is included, clearly this does not alter the problem; *i.e.,* (9) and (48) are equivalent. With either the IW or NN penalty included, (9) and (48) differ; whereas (9) encourages $\boldsymbol{U}_k/s_k$ to be close to $\boldsymbol{I}_R$, (48) encourages $\tilde{\boldsymbol{U}}_k/s_k$ to be close to $\boldsymbol{I}_R$, and in turn encourages $\boldsymbol{U}_k/s_k$ to be close to $\boldsymbol{V}$. Whether one or other is better is difficult to say in general, and may be context-dependent. Indeed, the transformation approach ensures a stronger version of the invariance property (7):

$$\hat{\theta}(\boldsymbol{A}\boldsymbol{x}, \boldsymbol{A}\boldsymbol{V}\boldsymbol{A}^T) = \boldsymbol{A}\hat{\theta}(\boldsymbol{x}, \boldsymbol{V}) \tag{49}$$

for any invertible matrix $\boldsymbol{A}$. Further (48) has the advantage that it can be solved by our TED approach when $\boldsymbol{V}_j = \boldsymbol{V} \neq \boldsymbol{I}_R$, whereas (9) cannot. We therefore take the transformation approach as the default approach in our software.

Note that, for the IW and NN penalties, the penalty term in (48) does not depend on the exact choice of matrix $\boldsymbol{R}$ in $\boldsymbol{V} = \boldsymbol{R}\boldsymbol{R}^T$. For example,

$$\begin{aligned}
\rho_\lambda^{\text{IW}}(\boldsymbol{R}^{-1}\boldsymbol{U}\boldsymbol{R}^{-T}) &= \frac{\lambda}{2}\left[\log\det \boldsymbol{R}^{-1}\boldsymbol{U}\boldsymbol{R}^{-T} + \text{tr}((\boldsymbol{R}^{-1}\boldsymbol{U}\boldsymbol{R}^{-T})^{-1})\right] \\
&= \frac{\lambda}{2}\left[\log\det \boldsymbol{U} + \log\det \boldsymbol{R}^{-1}\boldsymbol{R}^{-T} + \text{tr}(\boldsymbol{R}^T\boldsymbol{U}^{-1}\boldsymbol{R})\right] \\
&= \frac{\lambda}{2}\left[\log\det \boldsymbol{U}\boldsymbol{V}^{-1} + \text{tr}(\boldsymbol{U}^{-1}\boldsymbol{V})\right].
\end{aligned}$$

1.5. *Algorithms for a special case of the EBMNM model when $K = 1$.* In the M-step of Algorithm 1, we maximize the part of $F$ that depends on $\boldsymbol{U}_k$ for each $k$, which is (27):

$$\max_{\boldsymbol{U} \in P_R^{+,k},\, s>0} \phi(\boldsymbol{U}; \boldsymbol{w}_k) - \rho(\boldsymbol{U}/s), \tag{50}$$

where

$$\phi(\boldsymbol{U}; \boldsymbol{w}) := \sum_{j=1}^{n} w_j \log N_R(\boldsymbol{x}_j; \boldsymbol{0}, \boldsymbol{U} + \boldsymbol{V}_j).$$

We take an alternating optimization approach to solving (50) in which we alternate between maximizing over $\boldsymbol{U}$ with fixed $s$, and maximizing over $s$ with fixed $\boldsymbol{U}$. We have three algorithms to maximize over $\boldsymbol{U}$ in (50), which are detail in the following subsections. The update for $s$ is given in Section 1.5.4.

1.5.1. *Truncated eigenvalue decomposition.* We derive TED algorithm in the case where $\boldsymbol{V}_j = \boldsymbol{I}_R$. When $\boldsymbol{V} \neq \boldsymbol{I}_R$, we can simplify to the special case of $\boldsymbol{V}_j = \boldsymbol{I}_R$ by performing a simple data transformation described in Section 1.4. When $\boldsymbol{V}_j = \boldsymbol{I}_R$ for all $j$, $\phi$ in (26) simplifies. Specifically, dropping terms that do not depend on $\boldsymbol{U}$, we have

$$\phi(\boldsymbol{U}; \boldsymbol{w}) = -\frac{\bar{w}}{2}\left\{\log|\boldsymbol{U} + \boldsymbol{I}| + \text{tr}[(\boldsymbol{U} + \boldsymbol{I})^{-1}\hat{\boldsymbol{S}}]\right\}, \tag{51}$$

where $\boldsymbol{I} = \boldsymbol{I}_R$, and $\hat{\boldsymbol{S}} := \sum_{j=1}^n \tilde{w}_j \boldsymbol{x}_j \boldsymbol{x}_j^T$ is the (weighted) sample covariance with renormalized weights $\tilde{w}_j := w_j/\bar{w}$, $\bar{w} := \sum_{j=1}^n w_j$. Differentiating (51) with respect to $\boldsymbol{U} + \boldsymbol{I}$ and setting the derivative to zero yields the solution $\boldsymbol{U} = \hat{\boldsymbol{S}} - \boldsymbol{I}$. However, the matrix $\hat{\boldsymbol{S}} - \boldsymbol{I}$ is not necessarily a covariance; that is, it may have one or more eigenvalues that are negative. Intuitively, one might propose to create a valid covariance matrix by setting the negative eigenvalues to zero. Indeed, this intuition is correct: setting the negative eigenvalues of $\hat{\boldsymbol{S}} - \boldsymbol{I}$ to zero can be justified on the grounds that it maximizes (51) subject to the constraint that $\boldsymbol{U} \in P_R^+$. This is stated more formally by the following result.

RESULT 1. Let $\phi(\boldsymbol{U}; \boldsymbol{w})$ be defined in (51), and let $\hat{\boldsymbol{S}} = \boldsymbol{L}\boldsymbol{D}\boldsymbol{L}^T$ be the eigenvalue decomposition of $\hat{\boldsymbol{S}}$, with $\boldsymbol{D} := \mathrm{diag}(d_1, \ldots, d_R)$. Then we have that

$$\mathrm{argmax}_{\boldsymbol{U} \in P^+}\, \phi(\boldsymbol{U}; \boldsymbol{w}) = \boldsymbol{L}(\boldsymbol{D} - \boldsymbol{I})_+ \boldsymbol{L}^T, \tag{52}$$

where $\boldsymbol{A}_+$ denotes the matrix constructed from $\boldsymbol{A}$ by setting any negative elements of $\boldsymbol{A}$ to zero.

REMARK 1. It is straightforward to generalize this result to include an additional constraint on the rank of $\boldsymbol{U}$. Specifically, optimizing over $\boldsymbol{U}$ subject to the constraint that its rank is less than $R'$ (where $R' \leq R$) can be achieved by first setting all negative eigenvalues to zero, then, if needed, setting the smallest positive eigenvalues to zero until at least $R - R'$ eigenvalues are zero.

With the addition of a penalty, $\rho_\lambda^{\mathrm{IW}}(\boldsymbol{U})$ or $\rho_\lambda^{\mathrm{NN}}(\boldsymbol{U})$, the subproblem (27) no longer has a closed-form solution. However, it can nonetheless be solved easily using numerical methods, as explained in the following proposition.

PROPOSITION 2. Let $\rho(\boldsymbol{U})$ be a function of $R \times R$ matrix $\boldsymbol{U}$ that is separable in the eigenvalues of its argument; that is, $\rho(\boldsymbol{U}) = \sum_{r=1}^R \rho_r(e_r)$ for some $\rho_r(\cdot)$, in which $e_r$ denotes the $r$th eigenvalue of $\boldsymbol{U}$. (This separability property is satisfied by both the IW and NN penalties.) Then

$$\mathrm{argmax}_{\boldsymbol{U} \in P^+}\, \phi(\boldsymbol{U}; \boldsymbol{w}) - \rho(\boldsymbol{U}/s) = \boldsymbol{L}\mathrm{diag}(\hat{e}_1, \ldots, \hat{e}_R)\boldsymbol{L}^T, \tag{53}$$

where

$$\hat{e}_r := \underset{e_r \geq 0}{\mathrm{argmax}} -\frac{\bar{w}}{2}\left\{ \log(e_r + 1) + \frac{d_r}{e_r + 1} \right\} - \rho_r(e_r/s). \tag{54}$$

PROOF. The proof relies on the following result, which is a corollary to the Von NeumannâĂŞFan trace inequality (Mirsky, 1975), and is also used by Chi and Lange (2014):

RESULT 2. For Hermitian $n \times n$ positive semidefinite complex matrices $\boldsymbol{A}, \boldsymbol{B}$ where the eigenvalues are sorted in decreasing order, $a_1 \geq a_2 \geq \cdots \geq a_n$ and $b_1 \geq b_2 \geq \cdots \geq b_n$, respectively, we have

$$\sum_{i=1}^n a_i b_{n-i+1} \leq \mathrm{tr}(\boldsymbol{A}\boldsymbol{B}) \leq \sum_{i=1}^n a_i b_i, \tag{55}$$

with equality if and only if $\boldsymbol{A}$ and $\boldsymbol{B}$ share singular vectors.

We use Result 2 to prove the following lemma:

LEMMA 1. Define $f(\boldsymbol{Q},\boldsymbol{E};\boldsymbol{w}) := \phi(\boldsymbol{QEQ}^T;\boldsymbol{w})$ where $\phi$ denotes the function defined in (51), and $\boldsymbol{QEQ}^T$ is the eigenvalue decomposition of $\boldsymbol{U}$, so $\boldsymbol{Q}$ is an orthonormal matrix, and $\boldsymbol{E}$ is a diagonal matrix with non-negative entries $e_1 \geq e_2 \geq \ldots e_R \geq 0$ (so $\boldsymbol{QEQ}^T \in P_R^+$). Let $\boldsymbol{LDL}^T$ be the eigenvalue decomposition of the matrix $\boldsymbol{S}$ appearing in $\phi$. Then

$$\boldsymbol{L} = \underset{\boldsymbol{Q}}{\operatorname{argmax}}\, f(\boldsymbol{Q},\boldsymbol{E};\boldsymbol{w}), \tag{56}$$

and

$$\max_{\boldsymbol{Q}} f(\boldsymbol{Q},\boldsymbol{E};\boldsymbol{w}) = -\frac{\bar{w}}{2}\sum_{r=1}^{R}\left[\log(e_r+1) + \frac{d_r}{e_r+1}\right]. \tag{57}$$

PROOF. From the definition,

$$f(\boldsymbol{Q},\boldsymbol{E};\boldsymbol{w}) = -\frac{\bar{w}}{2}\left(\log|\boldsymbol{QEQ}^T + \boldsymbol{I}_R| + \operatorname{tr}((\boldsymbol{QEQ}^T + \boldsymbol{I}_R)^{-1}\boldsymbol{S})\right) \tag{58}$$

$$= -\frac{\bar{w}}{2}\left(\log|\boldsymbol{E} + \boldsymbol{I}_R| + \operatorname{tr}(\boldsymbol{Q}(\boldsymbol{E} + \boldsymbol{I}_R)^{-1}\boldsymbol{Q}^T\boldsymbol{S})\right) \tag{59}$$

so

$$\max_{\boldsymbol{Q}} f(\boldsymbol{Q},\boldsymbol{E};\boldsymbol{w}) = -\frac{\bar{w}}{2}\left[\sum_r \log(e_r+1) + \min_{\boldsymbol{Q}} \operatorname{tr}(\boldsymbol{Q}(\boldsymbol{E} + \boldsymbol{I}_R)^{-1}\boldsymbol{Q}^T\boldsymbol{S})\right]. \tag{60}$$

From (55) (left inequality), we have:

$$\operatorname{tr}(\boldsymbol{Q}(\boldsymbol{E} + \boldsymbol{I}_R)^{-1}\boldsymbol{Q}^T\boldsymbol{S}) \geq \sum_{i=1}^{R}\frac{d_i}{e_i+1}, \tag{61}$$

with equality if and only if $\boldsymbol{Q} = \boldsymbol{L}$, and the result follows. □

Proposition 2 then follows by parameterizing $\boldsymbol{U} = \boldsymbol{QEQ}^T$ and optimizing over $\boldsymbol{U}$ by optimizing over $\boldsymbol{Q}, \boldsymbol{E}$. □

REMARK 2. For separable penalties, the high-dimensional optimization problem (27) reduces to solving several 1-d optimization problems of the form (54). These 1-d optimization problems can be solved very efficiently using standard numerical algorithms. Result 1 follows as a simple corollary, by setting the penalty to zero and noting that the maximum of (54) is then $\hat{e}_r = \max\{0, d_r - 1\}$. Note that Tipping and Bishop (1999) proved a result similar to Result 1.

1.5.2. *Extreme Deconvolution.* The ED algorithm for solving (27) is due to Bovy, Hogg and Roweis (2011) and is indeed an EM algorithm for solving weighted log-likelihood based on the data augmentation representation (16). In this case, the weighted "complete data" log-likelihood is

$$\phi^{\text{ED}}(\boldsymbol{U},\boldsymbol{\Theta};\boldsymbol{w}) = \sum_{j=1}^{n} w_j \log p(\boldsymbol{x}_j, \boldsymbol{\theta}_j \mid \boldsymbol{U}, \boldsymbol{V}_j). \tag{62}$$

Following Proposition 1, the subproblem (27) can be solved by the following EM steps:

- E-step: compute the posterior mean and covariance of $\boldsymbol{\theta}_j$ given current estimate of $\boldsymbol{U}$:

$$\boldsymbol{b}_j = \boldsymbol{U}(\boldsymbol{U} + \boldsymbol{V}_j)^{-1}\boldsymbol{x}_j \tag{63}$$

$$\boldsymbol{B}_j = \boldsymbol{U} - \boldsymbol{U}(\boldsymbol{U} + \boldsymbol{V}_j)^{-1}\boldsymbol{U}. \tag{64}$$

- M-step:

$$\boldsymbol{U}^{\text{new}} \leftarrow \text{argmax}_{\boldsymbol{U}} \, E_{\boldsymbol{\Theta}|\boldsymbol{X}}\left[\phi^{\text{ED}}(\boldsymbol{U}, \boldsymbol{\Theta}; \boldsymbol{w})\right] - \rho(\boldsymbol{U}/s; \lambda). \tag{65}$$

Without a penalty, the ED update (65) has the following closed-form solution,

$$\boldsymbol{U}^{\text{new}} = \sum_{j=1}^{n} \tilde{w}_j(\boldsymbol{B}_j + \boldsymbol{b}_j\boldsymbol{b}_j^T), \tag{66}$$

where $\tilde{w}_j$ are the normalized weights, $\tilde{w}_j := w_j/\bar{w}$, $\bar{w} := \sum_{j=1}^{n} w_j$. With the IW penalty, the ED update also has a closed form, which is:

$$\boldsymbol{U}^{\text{new}} = \frac{\sum_{j=1}^{n} w_j(\boldsymbol{B}_j + \boldsymbol{b}_j\boldsymbol{b}_j^T) + \lambda s \boldsymbol{I}_R}{\sum_{j=1}^{n} w_j + \lambda}. \tag{67}$$

This expression is derived below. Under the NN penalty, the ED updates are not closed form, so we have not implemented them.

For simplicity, we have presented ED as solving the subproblem (27), which would involve iterating the updates (66) until they have converged to a stationary point (within some specified convergence tolerance). Practically speaking, however, iterating the ED updates typically suffer from "diminishing returns" in the sense that repeated updates make smaller and smaller improvements to the likelihood. Therefore, it is often more efficient to not try to solve the subproblem accurately, and perform only a few updates. In our implementation, we run ED for one iteration in each M-step of Algorithm 1. The same approach was adopted in Bovy, Hogg and Roweis (2011).

*Derivation for ED algorithm with IW penalty.* The M-step involves maximizing,

$$\begin{aligned} E\left[\phi^{\text{ED}}(\boldsymbol{U}, \boldsymbol{\Theta}, \boldsymbol{w}\right] - \rho^{IW}(\boldsymbol{U}/s) &= \sum_{j=1}^{n} w_j\big(-\frac{1}{2}\log|\boldsymbol{U}| - \frac{1}{2}\text{tr}[(\boldsymbol{B} + \boldsymbol{b}_j\boldsymbol{b}_j^T)\boldsymbol{U}^{-1}]\big) \\ &\quad - \frac{\lambda}{2}[\log|\boldsymbol{U}| - R\log s + \text{tr}(s\boldsymbol{U}^{-1})] + \text{constant}, \end{aligned} \tag{68}$$

where $\boldsymbol{B}$ and $\boldsymbol{b}_j$ are defined in (64) and (63). Denote the part of (68) that depends on $\boldsymbol{U}$ as $f(\boldsymbol{U})$. We take the (matrix) derivative of $f(\boldsymbol{U})$ with respect to $\boldsymbol{U}^{-1}$ and find the $\boldsymbol{U}^{-1}$ that sets the derivative to 0.

$$\frac{f(\boldsymbol{U})}{\partial \boldsymbol{U}^{-1}} = \frac{\sum_j^n w_j + \lambda}{2}\boldsymbol{U} - \frac{1}{2}\big(\sum_{j=1}^{n} w_j(\boldsymbol{B}_j + \boldsymbol{b}_j\boldsymbol{b}_j^T) + s\lambda\boldsymbol{I}\big) = \boldsymbol{0}. \tag{69}$$

This gives the closed-form solution

$$\boldsymbol{U}^{\text{new}} = \frac{\sum_{j=1}^{n} w_j(\boldsymbol{B}_j + \boldsymbol{b}_j\boldsymbol{b}_j^T) + \lambda s \boldsymbol{I}_R}{\sum_{j=1}^{n} w_j + \lambda}. \tag{70}$$

*Subspace-preserving property of ED.* Although the ED update is seemingly very general, it has an important limitation: the ED updates (66) have the property that they are "subspace preserving". While this limitation is not a big issue for unconstrained matrices, it makes ED poorly suited for estimating low-rank matrices, and in particular matrices with the rank-1 constraint; the ED updates (without penalty) will leave $\boldsymbol{U}$ unchanged aside from a change in scale. As far as we are aware, we are the first to report this limitation of ED. Fortunately, there is another iterative approach which is much better suited to updating covariances $\boldsymbol{U}$ with constraints on the rank of $\boldsymbol{U}$. This is described in the next section.

A feature of the ED algorithm is that, if $\boldsymbol{U}$ is initialized to a rank-1 matrix then the ED update does not change $\boldsymbol{U}$ (or only by a multiplicative constant). Thus the ED algorithm is not suited to estimating rank-1 matrices. More generally, the ED update does not change the column space of the matrix being updated.

This behavior can be seen directly from the form of the update (66), which can be written as $\boldsymbol{U}^{\text{new}} = \boldsymbol{U}\boldsymbol{A}$, where

$$\boldsymbol{A} := \sum_{j=1}^{n} \tilde{w}_j \left[(\boldsymbol{U} + \boldsymbol{V}_j)^{-1}\boldsymbol{x}_j\boldsymbol{x}_j^T(\boldsymbol{U} + \boldsymbol{V}_j)^{-1}\boldsymbol{U} + \boldsymbol{I} - (\boldsymbol{U} + \boldsymbol{V}_j)^{-1}\boldsymbol{U}\right]. \tag{71}$$

As a result, $\text{col}(\boldsymbol{U}^{\text{new}}) = \text{col}(\boldsymbol{U}\boldsymbol{A}) \subseteq \text{col}(\boldsymbol{U})$. The column space of $\boldsymbol{U}$ is defined as

$$\text{col}(\boldsymbol{U}) = \{\boldsymbol{y} \in \mathbb{R}^R : \boldsymbol{y} = \boldsymbol{U}\boldsymbol{x}, \boldsymbol{x} \in \mathbb{R}^R\}. \tag{72}$$

If $\boldsymbol{y}' \in \text{col}(\boldsymbol{U}\boldsymbol{A})$, we can find some $\boldsymbol{x}$ such that $\boldsymbol{y}' = \boldsymbol{U}\boldsymbol{A}\boldsymbol{x} = \boldsymbol{U}\boldsymbol{x}^*$, where $\boldsymbol{x}^* = \boldsymbol{A}\boldsymbol{x}$. Therefore $\text{col}(\boldsymbol{U}\boldsymbol{A}) \subseteq \text{col}(\boldsymbol{U})$.

1.5.3. *Factor analysis.* This last approach is motivated by our interest in fitting the EBMNM model with the restriction that some covariance matrices $\boldsymbol{U}_k$ are rank-1. This constraint was also used in Urbut et al. (2019), but they used a heuristic approach to estimate these rank-1 matrices.

To impose the rank-1 constraint, we reparameterize the covariance $\boldsymbol{U}$ as $\boldsymbol{U} = \boldsymbol{u}\boldsymbol{u}^T$, where $\boldsymbol{u} \in \mathbb{R}^R$. With this parameterization, the EBMNM subproblem becomes

$$\boldsymbol{x}_j \mid \boldsymbol{u}, \boldsymbol{V}_j \sim N_R(\boldsymbol{0}, \boldsymbol{u}\boldsymbol{u}^T + \boldsymbol{V}_j). \tag{73}$$

This model admits the augmented representation in (20). The weighted complete data log-likelihood in this case is:

$$\phi^{\text{FA}}(\boldsymbol{u}, \boldsymbol{a}; \boldsymbol{w}) = \sum_{j=1}^{n} w_j \log p(\boldsymbol{x}_j, a_j \mid \boldsymbol{u}, \boldsymbol{V}_j). \tag{74}$$

Following Proposition 1, the subproblem (27) can be solved by iteratively maximizing an expected (weighted) complete data log-likelihood,

$$\boldsymbol{u}^{\text{new}} = \text{argmax}_{\boldsymbol{u}} E_{a|\boldsymbol{X}}\left[\phi^{\text{FA}}(\boldsymbol{u}, a; \boldsymbol{w})\right], \tag{75}$$

in which the expectations are taken with respect to the posterior under model (20) at the current estimate of $\boldsymbol{u}$. (Recall, there is no penalty term because the rank-1 constraint is instead of a penalty.) The EM steps are the following:

1. E-step: Compute the posterior mean and variance of $a_j$, which are

$$\mu_j = \sigma_j^2 \boldsymbol{u}^T \boldsymbol{V}_j^{-1} \boldsymbol{x}_j \tag{76}$$

$$\sigma_j^2 = 1/(1 + \boldsymbol{u}^T \boldsymbol{V}_j^{-1} \boldsymbol{u}). \tag{77}$$

2. M-step: Maximize $\text{E}[\phi^{\text{FA}}(\boldsymbol{u}, \boldsymbol{a}; \boldsymbol{w})]$ with respect to $\boldsymbol{u}$, which has the closed-form solution

$$\boldsymbol{u}^{\text{new}} = \left(\sum_{j=1}^{n} w_j(\mu_j^2 + \sigma_j^2)\boldsymbol{V}_j^{-1}\right)^{-1}\left(\sum_{j=1}^{n} w_j\mu_j\boldsymbol{V}_j^{-1}\boldsymbol{x}_j\right). \tag{78}$$

1.5.4. *Updating the scaling parameter.* In the M-step of Algorithm 1, we update $s$ by maximizing the part that depends on $s$,

$$s^{\text{new}} = \underset{s>0}{\operatorname{argmax}} -\rho(\boldsymbol{U}/s). \tag{79}$$

For both the IW and NN penalties, the updates have closed-form solutions. For the IW penalty, the update is

$$s^{\text{new}} = \frac{R}{\text{tr}(\boldsymbol{U}^{-1})}. \tag{80}$$

For the NN penalty, the update is

$$s^{\text{new}} = \sqrt{\frac{\text{tr}(\boldsymbol{U})}{\text{tr}(\boldsymbol{U}^{-1})}}. \tag{81}$$

PROOF. For the IW penalty, based on (10), we have

$$\begin{aligned} \rho_\lambda^{\text{IW}}(\boldsymbol{U}/s) &= \frac{\lambda}{2}\left[\log|\boldsymbol{U}/s| + \text{tr}\big((\boldsymbol{U}/s)^{-1}\big)\right] \\ &= \frac{\lambda}{2}\left[\sum_{r=1}^{R}\log e_r - R\log s + s\text{tr}(\boldsymbol{U}^{-1})\right]. \end{aligned} \tag{82}$$

Taking the first derivative of $\rho_\lambda^{\text{IW}}(\boldsymbol{U}/s)$ with respect to $s$ and set it to zero, we obtain (80).

For the NN penalty, based on (12), we have

$$\begin{aligned} \rho_\lambda^{\text{NN}}(\boldsymbol{U}/s) &= \frac{\lambda}{2}\big(0.5\|\boldsymbol{U}/s\|_* + 0.5\|(\boldsymbol{U}/s)^{-1}\|_*\big) \\ &= \frac{\lambda}{2}\big(\frac{0.5}{s}\text{tr}(\boldsymbol{U}) + 0.5s\text{tr}(\boldsymbol{U}^{-1})\big). \end{aligned} \tag{83}$$

Taking the first derivative of $\rho_\lambda^{\text{NN}}(\boldsymbol{U}/s)$ with respect to $s$ and setting it to zero, and requiring $s > 0$, we obtain (81). □

1.5.5. *Updating $\boldsymbol{U}$ with a scaling constraint.* For the scaling constraint, in which $\boldsymbol{U} = c\boldsymbol{U}_0$ such that $\boldsymbol{U}_0$ is specified and $c > 0$ is the scalar parameter to be estimated, it is straightforward to solve the subproblem (25) by standard numerical methods for 1-d optimization.

1.6. *Proof that changing $\alpha$ is equivalent to changing $\lambda$ with scale invariance in the nuclear norm penalty.* Let's compute $\hat{s}$ using the original form of the NN penalty from Chi and Lange (2014):

$$\begin{aligned} \hat{s} &= \underset{s>0}{\operatorname{argmin}}\, \rho_\lambda^{\text{NN}}(\boldsymbol{U}/s;\alpha) \\ &= \underset{s>0}{\operatorname{argmin}}\, \frac{\lambda}{2}\big[\frac{\alpha}{s}\|\boldsymbol{U}\|_* + (1-\alpha)s\|\boldsymbol{U}^{-1}\|_*\big]. \end{aligned} \tag{84}$$

This results in

$$\hat{s} = \sqrt{\frac{\alpha\text{tr}(\boldsymbol{U})}{(1-\alpha)\text{tr}(\boldsymbol{U}^{-1})}}. \tag{85}$$

This computation is similar to 81. Plugging $\hat{s}$ into $\rho_\lambda^{\text{NN}}(\boldsymbol{U}/s;\alpha)$, we can see the term that includes $\alpha$ can be absorbed into $\lambda$:

$$\rho_\lambda^{\text{NN}}(\boldsymbol{U}/\hat{s};\alpha) = -\lambda\sqrt{(1-\alpha)\alpha}\sqrt{\text{tr}(\boldsymbol{U})\text{tr}(\boldsymbol{U}^{-1})}. \tag{86}$$

1.7. *Power and FSR.* Given an effect estimate $\hat{\theta}_{jr}$ and $lfsr_{jr}$ for each observation $j = 1, \ldots, n$ and dimension $r = 1, \ldots, R$, we define S as the set of significant effects at threshold $t \geq 0$, CS as the set of "correctly signed" results, T as the set of true nonzero effects, and N the set of true null (zero) effects:

$$\mathrm{S} = \{j, r : lfsr_{jr} \leq t\} \tag{87}$$

$$\mathrm{CS} = \{j, r : \hat{\theta}_{jr} \times \theta_{jr} > 0\} \tag{88}$$

$$\mathrm{N} = \{j, r : \theta_{jr} = 0\} \tag{89}$$

$$\mathrm{T} = \{j, r : \theta_{jr} \neq 0\}. \tag{90}$$

Then we define true positive rate (power) and false sign rate (FSR) at *lfsr* threshold $t$ as

$$\mathrm{TPR} = \frac{|\mathrm{CS} \cap \mathrm{S}|}{|\mathrm{T}|} \tag{91}$$

$$\mathrm{FSR} = \frac{|\mathrm{S}| - |\mathrm{CS} \cap \mathrm{S}|}{|\mathrm{S}|}. \tag{92}$$

## REFERENCES


BOVY, J., HOGG, D. W. and ROWEIS, S. T. (2011). Extreme Deconvolution: Inferring complete distribution functions from noisy, heterogeneous and incomplete observations. *Annals of Applied Statistics* **5** 1657–1677.

CHI, E. C. and LANGE, K. (2014). Stable estimation of a covariance matrix guided by nuclear norm penalties. *Computational statistics and Data Analysis* **80** 117–128.

MIRSKY, L. (1975). A trace inequality of John von Neumann. *Monatshefte für mathematik* **79** 303–306.

NEAL, R. and HINTON, G. (1998). A view of the EM algorithm that justifies incremental, sparse, and other variants. In *Learning in Graphical Models* (M. I. Jordan, ed.) 355–368. Springer, New York.

TIPPING, M. E. and BISHOP, C. M. (1999). Probabilistic principal component analysis. *Journal of the Royal Statistical Society, Series B* **61** 611–622.

URBUT, S. M., WANG, G., CARBONETTO, P. and STEPHENS, M. (2019). Flexible statistical methods for estimating and testing effects in genomic studies with multiple conditions. *Nature Genetics* **51** 187–195.

## Supplementary tables.

SUPPLEMENTARY TABLE 1

Computational complexity for homoskedastic case (when $\boldsymbol{V}_j = \boldsymbol{V}$). Per-iteration computational complexity of different algorithms for solving the subproblem when $n$ is much larger than $R$. $p$ is the rank of the canonical covariance matrix, $p \leq R$.

| | Unconstrained | Scaled | Rank-1 |
|---|---|---|---|
| TED | $O(R^3 + nR^2)$ | – | $O(R^3 + nR^2)$ |
| FA | $O(R^3 + nR^2)$ | $O(npR)$ | $O(nR)$ |
| ED | $O(R^3 + nR^2)$ | – | – |

SUPPLEMENTARY TABLE 2

Computational complexity for heteroskedastic case (when $\boldsymbol{V}_j$ varies). Per-iteration computational complexity of different algorithms for solving the subproblem when $n$ is much larger than $R$, in the case where $\boldsymbol{V}_j = \boldsymbol{I}$ and $\boldsymbol{V}_j$ varies. $p$ is the rank of the canonical covariance matrix, $p \leq R$. Note that TED algorithm doesn't work for the heteroskedastic case.

| | Unconstrained | Scaled | Rank-1 |
|---|---|---|---|
| ED | $O(nR^3)$ | – | – |
| FA | – | $O(npR^2)$ | $O(R^3 + nR^2)$ |

## Supplementary figures.

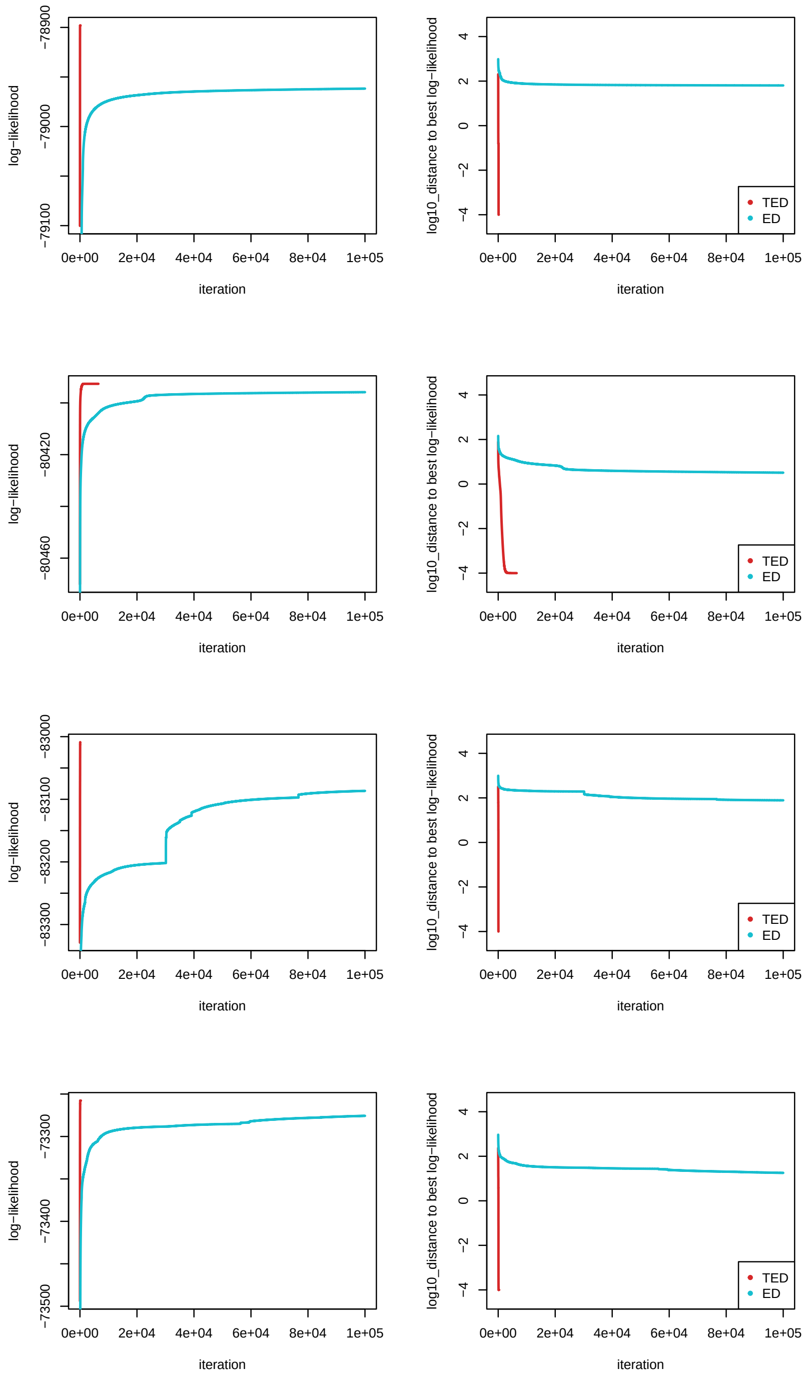


SUPPLEMENTARY FIGURE 1. Data examples for comparing the convergence between TED and ED. Each row represents one data example. We ran both algorithms for 100,000 iterations after running ED for 20 iterations initially.

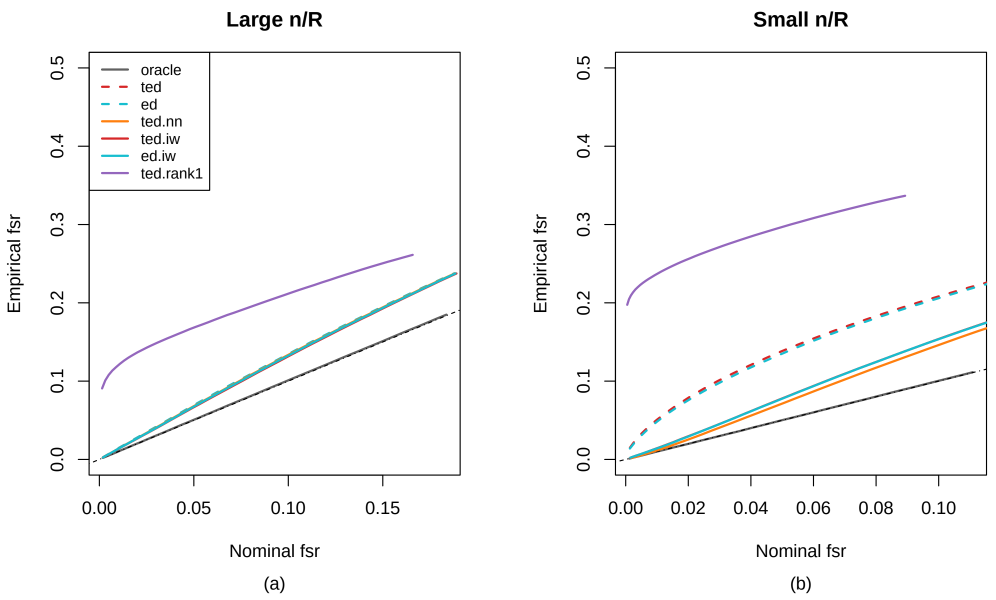


SUPPLEMENTARY FIGURE 2. Calibration of FSR for hybrid scenario. Other simulation parameters are as in Figure 4 in the main text. The dashed, black line represents the empirical FSR equals to nominal FSR.

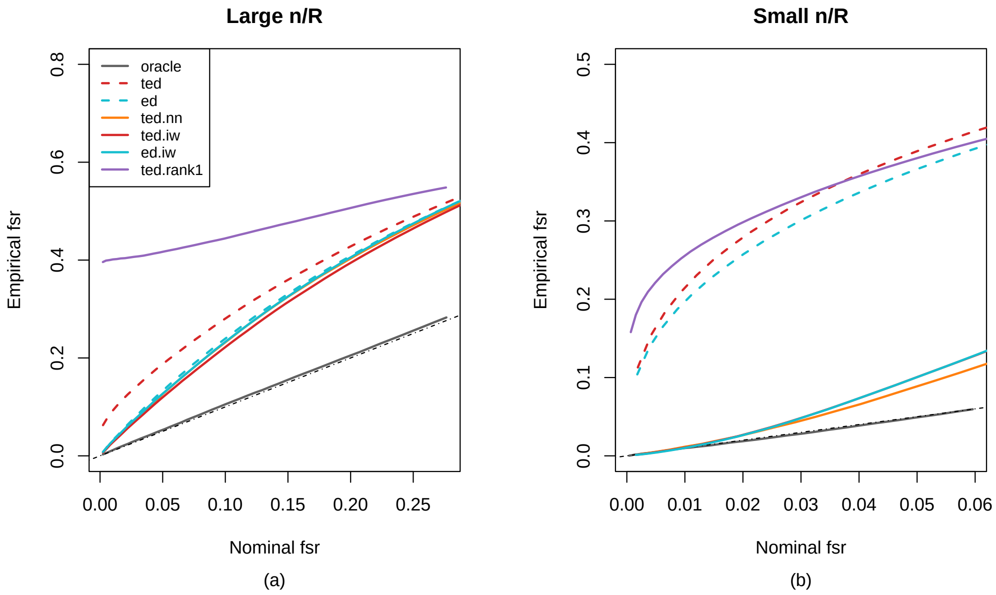


SUPPLEMENTARY FIGURE 3. Calibration of FSR where true covariances are all rank-1 matrices. Other simulation parameters are the same as Figure 5 in the main text. The dashed, black line represents empirical FSR equals the nominal FSR.

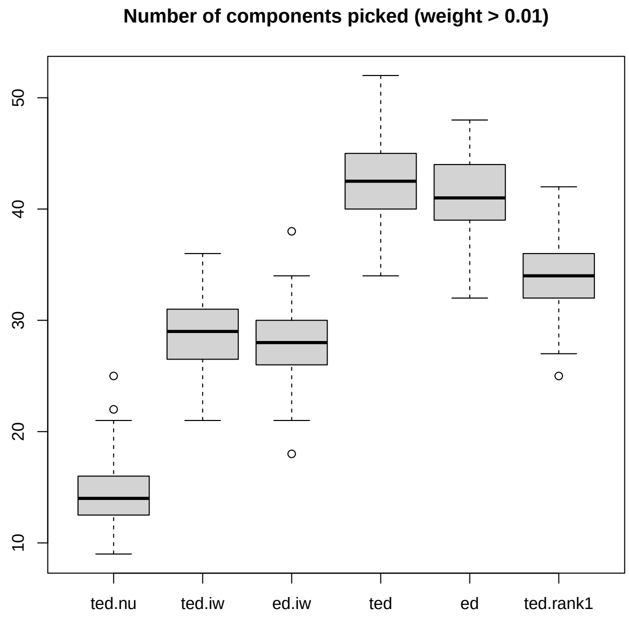


SUPPLEMENTARY FIGURE 4. The number of "important" components, defined as the components $k$ with mixture weight $\pi_k > 0.01$. (The true $K$ was 10.) Boxplots are based on 100 data replicates. For each simulated data set, $n = 1000$ and $R = 50$.
